# Supplementary material for: The maximum distinctness of physical systems
Source: arXiv:2111.00297 ancillary file (2025-07-23)
Supplement: Supplementary file 1 [file distinctness.nb.pdf]

# Verification of distinctness bounds using linear optimization

This notebook contains *Mathematica* code for numerical experiments used to investigate and verify bounds on counts of distinct states in a unitary evolution and to generate figures for the paper, “Counting distinct states in physical dynamics” (N. Margolus). The entire notebook takes about nine hours to evaluate on an iMac Pro (2017) with ten cores and 64GB of RAM using Mathematica 12.1.1.0.

The minimization and maximization problems outlined in the paper require determination of square magnitudes  $a_n = |c_n|^2$  of coefficients  $c_n$  in energy-basis superpositions  $|\psi(t)\rangle = \sum c_n e^{-2\pi i v_n t} |E_n\rangle$ ; the coefficients themselves never appear in our calculations. Similarly, only frequency differences ever appear in the problems, and so we take  $v_0 = 0$  without loss of generality; the allowed frequencies in an evolution of period  $T$  are  $v_n = n/T$ . For testing the bounds on generalized average deviations from frequency  $\alpha$ , which are defined as  $\langle v - \alpha \rangle_M \equiv (\sum a_n |v_n - \alpha|^M)^{1/M}$ , both the dimensionless objective function  $(T \langle v - \alpha \rangle_M)^M$  and all of the orthogonality constraints  $\langle \psi(t_m) | \psi(t_k) \rangle = \delta_{mk}$  are linear combinations of the  $a_n$ 's so, given any set of integer separations between distinct states, we can always find the global minimum numerically to any desired accuracy using linear optimization (linear programming). Here we only study the cases  $\alpha = v_0$  (deviations from the minimum) and  $\alpha = \bar{v}$  (deviations from the mean). We also use linear optimization to maximize sums of probabilities in a range of frequencies to study some non-deviation widths. In our analyses, all times are specified as integers, which ensures there are always a finite number of distinct phases in constraints, and hence a finite number of  $a_n$ 's required in the minimization computations: the integer period  $T$  of an entire recurrent evolution is the maximum number of  $a_n$ 's needed. Since there is no bound on  $T$ , the fraction of the total time represented by the separation between two distinct states can have any required resolution.

We first study average deviation widths, finding an assignment of  $a_n$ 's that give the minimum width for a randomly chosen set of time-separations between distinct states. We verify numerically that spreading a given number of distinct states evenly within a given period of periodic evolution allows smallest widths. We similarly verify that, for a given number of distinct states within a portion of evolution, equal separations there allow the complete evolution with the smallest possible width. Then, assuming equal separations are optimal, we compare numerical and theoretical bounds and show they exactly match. We also illustrate the convergence of numerical minima to limiting values for portions of an evolution, as the period of the full evolution the portion is part of grows larger. Finally, we numerically study a different example of a well-behaved frequency width: the width of frequency range needed to hold a given total probability, for evolutions that traverse a given number of distinct states. This helps establish that, for a periodic or unbounded evolution, any well-behaved frequency width

obeys distinctness bounds defined by a uniform minimum-bandwidth frequency distribution.

Additional numerical tests used to study generalized deviations and to evaluate the effectiveness of various methods of studying distinctness bounds can be found on [arxiv.org](https://arxiv.org) as ancillary material for “The finite-state character of physical dynamics”, arXiv:1109.4994, cited as reference [65] in that paper.

```
beginTime = AbsoluteTime[];
```

## Generalized Average Deviations

The average deviations  $\langle v - \alpha \rangle_M$  are a generalization of the standard deviation to other moments, and include deviations from the minimum and deviations from the mean. We define deviation widths to be twice average deviations. Well-known bounds on orthogonal evolution between two distinct states are special cases of more general distinctness bounds on these more general deviation widths.

---

### Minimize deviation widths, subject to constraints

Our basic tool for studying generalized deviations is the function **minimizeTM**, which takes a list of separation intervals and finds (square magnitude) coefficients  $a_n$  for an energy-basis superposition that minimizes  $T \langle v - \alpha \rangle_M$  for that list, returning the minimum value. The complete solution, including all coefficients  $a_n$ , is recorded in the global variable **soln**. Within this calculation, all times are rescaled so that total period  $T=1$ ; using this unit of time, a sorted list of all intervals between orthogonal states is stored in **deltaList**. For deviations about  $\alpha = \bar{v}$ , **minimizeTM** searches for the choice of  $\bar{v}$  that gives the smallest minimum, performing **osdMax** minimization steps trying different choices.

#### Construct arguments for NMinimize

|           |                                                                                             |
|-----------|---------------------------------------------------------------------------------------------|
| problem   | specification of the problem to be solved                                                   |
| momTM     | dimensionless objective function $(T \langle v - \alpha \rangle_M)^M$ , linear in the $a_n$ |
| asum      | constraint: coefficients must add to one                                                    |
| apos      | constraint: coefficients must be positive                                                   |
| acos      | orthogonality constraints: real parts                                                       |
| asin      | orthogonality constraints: imaginary parts                                                  |
| ntot      | number of coefficients used in minimization                                                 |
| $a_n$     | squared magnitude of n-th coefficient                                                       |
| vars      | list of all coefficients $a_n$ to be solved for                                             |
| deltaList | list of intervals between distinct states, taking $T$ as the unit of time                   |
| origin    | the frequency $\alpha$ about which deviations are minimized                                 |
| moment    | moment number $M$ of the deviation width                                                    |
| unsetA    | make sure all $a_n$ are unset, to use as symbolic variables                                 |

```

problem := Flatten[{momTM, asum, apos, acos, asin}];
momTM := Sum[an Abs[n - origin]moment, {n, 0, ntot - 1}];
asum := {Sum[an, {n, 0, ntot - 1}] == 1};
apos := Table[an ≥ 0, {n, 0, ntot - 1}];
acos := Table[{Sum[an Cos[2 Pi n deltaList[[k]]], {n, 0, ntot - 1}] == 0},
  {k, 1, Length[deltaList]}];
asin := Table[{Sum[an Sin[2 Pi n deltaList[[k]]], {n, 0, ntot - 1}] == 0},
  {k, 1, Length[deltaList]}];
vars := {unsetA; Array[Subscript[a, # - 1] &, ntot]};
unsetA := Do[{an = 0; an = .}, {n, 0, ntot - 1}];

```

### Minimize $T \langle v - \alpha \rangle_M$

minimizeTM    minimize width about  $v_0$  or  $\bar{v}$ , given a moment number and a list of separations  
 soln            soln[[1]] is minimum found by **minimizeTM**, soln[[2]] the minimizing set of  $a_n$   
 deltaT         deviation from origin, times the period  $T$   
 tauList        intervals between adjacent distinct states, taking  $T$  as the unit of time  
 findMin        calls **NMinimize**, adjusting **WorkingPrecision** if necessary  
 extraPrecision determines **WorkingPrecision** in **findMin** (global parameter)  
 osdMax         max search degree for finding best **origin** for moments about  $\bar{v}$  (global parameter)

```

minimizeTM[about_, momentM_, tauListM_, numC_ : 0] :=
Module[{middle, solnNum, solnList},
  tauList = tauListM / Total[tauListM]; moment = momentM;
  ntot = If[numC > 0, numC, LCM@@Denominator[tauList]]; (* drop common factor *)
  deltaList = Sort[DeleteDuplicates[Flatten[Table[Min[d = (t[m] - t[k]), 1 - d],
    {k, 0, Length[tauList] - 2}, {m, k + 1, Length[tauList] - 1}]]]];
  origin = If[about == aboutMean, (ntot - 1) / 2, 0]; soln = findMin;
  If[about == aboutMean, Do[{middle = origin;
    solnList = {origin = middle - 2-osd;
      findMin, soln, origin = middle + 2-osd; findMin};
    soln = solnList[[solnNum = Ordering[Table[solnList[[n]][[1]],
      {n, 1, 3}], 1][[1]]]]; origin = middle + (solnNum - 2) 2-osd;},
    {osd, 1, osdMax}]]; (* no search if osdMax=0 *)
  deltaT]

```

**findMin** uses the built in function **NMinimize**. Here the objective function and the constraints are both linear in the variables  $a_n$ , and in this case **NMinimize** will use linear optimization to find an assignment of the variables that achieves the global minimum (with linear optimization, a local minimum is always a global minimum).

```

extraPrecision = 0; osdMax = 1; (* Defaults. Restore if changed!! *)
findMin := If[extraPrecision <= 0, NMinimize[problem, vars, PrecisionGoal → 6],
  NMinimize[problem, vars, WorkingPrecision → extraPrecision, PrecisionGoal → 6]]

```

```

deltaT := ((soln[[1]])^(1/moment));
tau[n_] := tauList[(Mod[n, Length[tauList]] + 1)];
t[n_] := Sum[tau[k], {k, 0, n - 1}];
aboutMean = True;
aboutMin = False;

```

As a simple usage example, we compare numerical minima of  $\tau \Delta v$  for  $N$  equally separated distinct states with theoretical values for deviation widths  $\Delta v$ , defined to be twice the deviation. **minimizeTM** minimizes period times deviation,  $T \Delta v/2$ , so multiplying by  $2 \tau/T = 2/N$  gives the minimum for  $\tau \Delta v$ .

```

fMin[moment_, distinct_] := 2 distinct^(- (1 + 1/moment)) (Sum[n^moment, {n, 0, distinct - 1}])^(1/moment);
fMean[moment_, distinct_] :=
  2 distinct^(- (1 + 1/moment)) (Sum[Abs[n - distinct/2]^moment, {n, 0, distinct - 1}])^(1/moment);

Table[{N[fMin[1, n]], (2/n) minimizeTM[aboutMin, 1, Table[1, n]]}, {n, 2, 10}]
{{0.5, 0.5}, {0.666667, 0.666667}, {0.75, 0.75}, {0.8, 0.8}, {0.833333, 0.833333},
 {0.857143, 0.857143}, {0.875, 0.875}, {0.888889, 0.888889}, {0.9, 0.9}}

Table[{N[fMean[1, n]], (2/n) minimizeTM[aboutMean, 1, Table[1, n]]}, {n, 2, 10}]
{{0.5, 0.5}, {0.444444, 0.444444}, {0.5, 0.5}, {0.48, 0.48}, {0.5, 0.5},
 {0.489796, 0.489796}, {0.5, 0.5}, {0.493827, 0.493827}, {0.5, 0.5}}

```

## Plot overlap $\langle \psi(t) | \psi(0) \rangle$ for **minimizeTM** minimizing state

We also define the functions **makeOverlap** and **plotOverlap**, which allow a minimizing state found by **minimizeTM** (recorded in global variable **soln**) to be studied in detail. **makeOverlap** uses **soln** to create a function **overlap** that evaluates the overlap  $\langle \psi(t) | \psi(0) \rangle$  of the minimizing state for given  $t$ , returning a vector of terms of the overlap with non-zero coefficients. **plotOverlap** uses this function to plot either the magnitude or the real and imaginary parts of the overlap for a given portion of the period.

|                    |                                                                                                              |
|--------------------|--------------------------------------------------------------------------------------------------------------|
| <b>makeOverlap</b> | defines a function <b>overlap</b> using <b>soln</b> , creating auxiliary lists <b>pList</b> and <b>cList</b> |
| <b>overlap</b>     | given $t$ , returns a vector of all non-zero terms of the overlap $\langle \psi(t)   \psi(0) \rangle$        |
| <b>pList</b>       | list of positions of non-zero coefficients                                                                   |
| <b>cList</b>       | list of rules for assigning non-zero coefficients                                                            |
| <b>plotOverlap</b> | plot either magnitude or real + imaginary parts of overlap, with labels                                      |
| <b>realRep</b>     | returns either the magnitude or list of {real,imaginary} parts of a complex value                            |

```

makeOverlap := (unsetA;
  pList = Position[Map[Function[x, x > 10^(-20)], (vars /. soln[[2])]], True];
  cList = Extract[soln[[2]], pList];
  overlap =
    Block[{dt, n}, Function[dt, Evaluate[(pList - 1 /. {n_} → a_n E^(2 π i n dt) /. cList)]];

plotOverlap[tMin_, tMax_, tFull_, absP_, opts : OptionsPattern[]] :=
  (Plot[Evaluate[realRep[Total[overlap[t/tFull]], absP]], {t, tMin, tMax},
    Evaluate[FilterRules[{opts}, Options[Plot]]],
    AxesOrigin → {tMin, 0}, AxesLabel →
      {Style["t"], If[absP, Style["|⟨ψ(t) | ψ(0)⟩|"], Style["⟨ψ(t) | ψ(0)⟩"]]},
    PlotStyle → Directive[Thickness[.004], If[absP, Blue, {Blue, Dashed}]]];

realRep[z_, absP_] := If[absP, Abs[z], {Re[z], Im[z]}];
showMag = True;
showParts = False;

```

For example, suppose we use **minimizeTM** to find the smallest  $\Delta v T$  for the first-deviation from the minimum with 4 equally separated distinct states. The width  $\Delta v T$  is dimensionless, but if we take the average separation between adjacent distinct states as our unit of time ( $t_{Full} = 4$ ), the magnitude of overlap  $\langle \psi(t) | \psi(0) \rangle$  of initial state and later state looks like this over time:

```

minimizeTM[aboutMin, 1, {1, 1, 1, 1}]; makeOverlap;
plotOverlap[0, 4, 4, showMag, Ticks → {Range[4], Automatic}, ImageSize → 250]

```

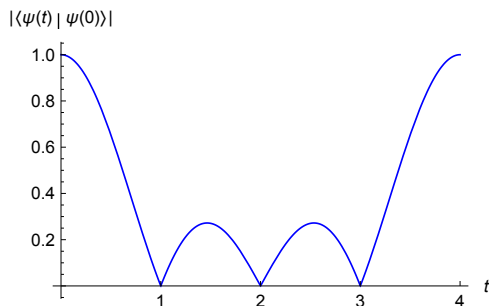

In order to have orthogonality between four distinct states, the overlap must be zero at separations of 1, 2, and 3. The list of orthogonal separations used by the most recent minimization, **deltaList**, is stored as fractions of the total period, so we restore it to integer form by multiplying by the least common denominator for the list:

```

deltaList LCM@@Denominator[deltaList]
{1, 2}

```

In this case the list has only two entries, since orthogonality is symmetric in time: for a period 4 evolution, zero-overlap at separation +3 is the same as zero-overlap at separation -1.

## Equal vs unequal separations for periodic evolutions

We verify that, if we only know that there are  $N$  distinct states in an entire periodic evolution of length  $T$ , the minimum deviation widths are always smallest if the states are uniformly spaced in time. We do this by experimentally determining how minimum widths vary with the number  $K_{\text{different}}$  of different separation lengths in period  $T$ . We find that the minimum possible widths increase in discrete jumps as  $K_{\text{different}}$  increases, so the global minimum is always obtained with equal separations.

To determine the minimum for a randomly chosen set of separations we define **minimizeSet**, which tests a specified set of separations. We then define **randTauList** to generate a list stochastically that contains  $K_{\text{different}} = 2, 3$ , or 4 different separation lengths, each an integer up to 100, with each set having up to 12 separations in all. In generating the random set of separations, half of the time we weight longer separations more highly, since we find that these sets yield lower minima. The rest of the time all weights are equal. Much longer experiments give the same results.

```
minimizeSet[about_, moment_, tauList_] := Block[{et, osdMax = 8},
  {tauList, et = Table[1, Length[tauList]], Length[DeleteDuplicates[tauList]],
    -2 minimizeTM[about, moment, et] + 2 minimizeTM[about, moment, tauList]}}

randTau :=
  If[RandomInteger[1] == 0, RandomInteger[{1, 100}], RandomInteger[{95, 100}]];

randDiffList[kdiff_] := While[True, Module[{diff},
  diff = Table[randTau, {kdiff}];
  diff = DeleteDuplicates[diff];
  If [Length[diff] == kdiff, Return[Sort[diff]]]]]

randTauList[kdiff_] := Module[{diff},
  diff = randDiffList[kdiff];
  RandomSample[Flatten[Table[diff[[n]], {n, 1, Length[diff]}],
    {If[RandomInteger[{1, 5}] < 5, 1, RandomInteger[{2, 3}]]}]]]
```

For example, in

```
minimizeSet[aboutMin, 1, randTauList[3]]
{{98, 98, 84, 98, 96}, {1, 1, 1, 1, 1}, 3, 4.39772}
```

we see that **minimizeSet** returns a list with four elements: a randomly generated set of separations, a set of the same length with equal separations, the number of different separations in the first list, and the difference of minima for the two cases. Since we are minimizing a dimensionless quantity  $T \Delta v$ , we can think of the period  $T$  as always normalized to one, minimizing  $\Delta v$  with that normalization. Thus using bigger integers for separations just allows us to increase the resolution of the relative lengths.

**minimizeSets** repeats **minimizeSet** *numSets* times, to construct a list of four element lists, and then prints out execution time.

```

minimizeSets[about_, moment_, kdiff_, numSets_] := Module[{start, table},
  start = AbsoluteTime[];
  table = sortLast[ParallelTable[minimizeSet[about, moment, randTauList[kdiff]],
    {numSets}], Method → "FinestGrained"];
  Print["Execution took ", Round[(AbsoluteTime[] - start) / 60, .001], " minutes"];
  table]

```

**sortLast** sorts list of lists by the last entry in each top level element, dropping elements where the last entry has no digits of precision.

```

sortLast[list_] := Module[{slist = SortBy[list, Last], rlist = {}},
  Do[If[Precision[Last[slist[[n]]]] ≥ 1, AppendTo[rlist, slist[[n]]],
    {n, Length[slist]}]; rlist]

```

**last2** drops part of each top-level element of *list*, keeping just last two components of each element.

```
last2[list_] := Map[Function[u, u[[-2 ;; -1]]], list];
```

Here's a usage example for **minimizeSets**. Results appear sorted by the width value at the end of each element.

```
smallTest = minimizeSets[aboutMin, 1, 3, 6]
```

```
Execution took 0.032 minutes
```

```

{{{57, 98, 72}, {1, 1, 1}, 3, 2.49609},
 {{96, 42, 99}, {1, 1, 1}, 3, 3.12145}, {{24, 94, 68}, {1, 1, 1}, 3, 4.},
 {{99, 95, 95, 95, 84}, {1, 1, 1, 1, 1}, 3, 4.2889}, {{11, 48, 39}, {1, 1, 1}, 3, 4.68564},
 {{35, 35, 100, 35, 99, 100}, {1, 1, 1, 1, 1, 1}, 3, 7.86611}}

```

```
last2[smallTest]
```

```
{{3, 2.49609}, {3, 3.12145}, {3, 4.}, {3, 4.2889}, {3, 4.68564}, {3, 7.86611}}
```

## Deviations from the minimum

Now we run an experiment for the first moment about a minimum frequency. We adjust the number of samples tested for each value of  $K_{\text{different}}$  to get an even density when we plot the results.

```
min2 = minimizeSets[aboutMin, 1, 2, 5000];
```

```
Execution took 0.202 minutes
```

```
min3 = minimizeSets[aboutMin, 1, 3, 2000];
```

```
Execution took 0.204 minutes
```

```
min4 = minimizeSets[aboutMin, 1, 4, 5000];
```

```
Execution took 1.112 minutes
```

If we look at the minimum value of  $T\Delta v$  for each number  $K_{\text{different}} > 1$  of different separation lengths seen in a long experiment, we find that the minimum is achieved by  $K_{\text{different}}$  different integers that are as close to being equal as is possible (in ratio), given that we only use integers up to 100. In fact that is

what we always find in sufficiently long experiments using other deviation widths.

```
minList = {min2[[1]], min3[[1]], min4[[1]]};
```

```
last2[minList]
```

```
{{2, 1.}, {3, 2.02008}, {4, 3.0625}}
```

```
Map[First, minList]
```

```
{{47, 44}, {98, 99, 100}, {98, 99, 97, 100}}
```

$K_{\text{different}} = 2$  is a special case where *many different pairs of unequal separations have exactly the same minimum*, one unit higher than equal separations; minima may appear unequal due to imprecision.

```
Block[{extraPrecision = 1000},
```

```
  Last[minimizeSet[aboutMin, 1, {99, 100}] - minimizeSet[aboutMin, 1, {44, 41}]]]
```

```
0.  $\times 10^{-995}$ 
```

We compute a few extra minima corresponding to almost-equal cases with higher resolution (larger integer numbers for the separations, allowing the values to be proportionately closer), so that our plot can include these cases as well.

```
aeqN[about_, moment_, distinct_] :=
```

```
  Table[minimizeSet[about, moment, Range[4 k2, 4 k2 + distinct - 1]], {k, 6, 8}];
```

```
aeqList[about_, moment_, maxDistinct_, start_ : 1000] :=
```

```
  Table[minimizeSet[about, moment, Range[start, start + n - 1]], {n, 1, maxDistinct}];
```

```
last2[aeqList[aboutMin, 1, 4]]
```

```
{{1, 0.}, {2, 1.}, {3, 2.00199}, {4, 3.00592}}
```

```
minXPlot = ListPlot[
  last2[Join[aeqList[aboutMin, 1, 4], aeqN[aboutMin, 1, 4], min2, min3, min4]],
  PlotRange → {- .1, 3.8}, PlotStyle → Black, Ticks → {Range[4], Automatic},
  PlotMarkers → Graphics[{Thickness[.01], Line[{{- .05, 0}, {.05, 0}]}]},
  AxesLabel → {Style[" $K_{\text{different}}$ ", 16], Style[" $T(\Delta\nu_{1,\text{min}} - \Delta\nu_{\text{equal}})$ ", 16]},
  ImageSize → 500]
```

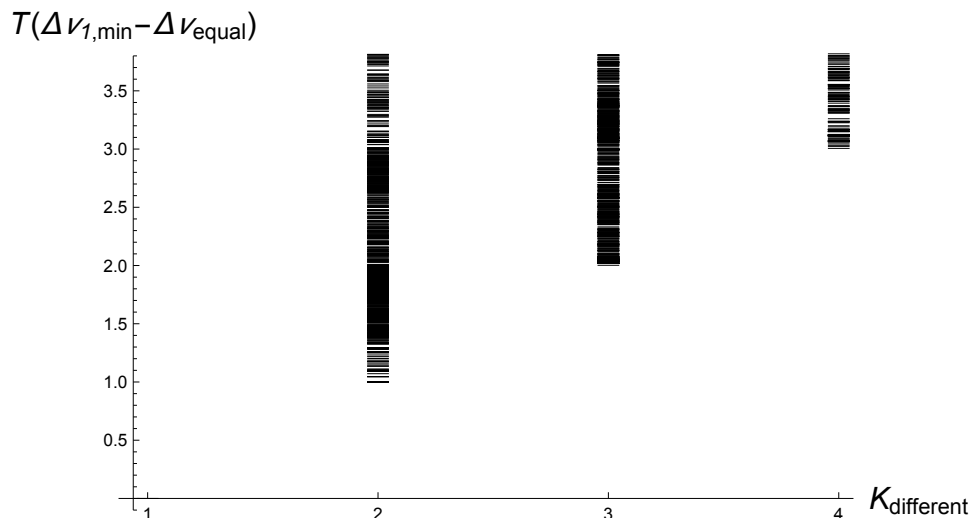

The smallest minima of  $T(\Delta\nu_{1,\text{min}} - \Delta\nu_{\text{equal}})$  for evolutions with different numbers of different separations  $K_{\text{different}}$  lie on a straight line. Equal separations ( $K_{\text{different}}=1$ ) always give the global minimum.

## Limiting behavior

We can understand the limiting behavior of almost-equal separations by looking at an example. Consider three almost-equal separations {99, 100, 101} in a periodic evolution with three distinct states.

```
minimizeTM[aboutMin, 1, {99, 100, 101}]; make0overlap;

{ε = 2; plotOverlap[0, 300, 300, showMag, Ticks → {100 Range[3], Automatic}],
 plotOverlap[100 - ε, 100 + ε, 300, showMag, Ticks → {Range[101], Automatic}],
 plotOverlap[200 - ε, 200 + ε, 300, showMag, Ticks → {Range[201], Automatic}]}
```

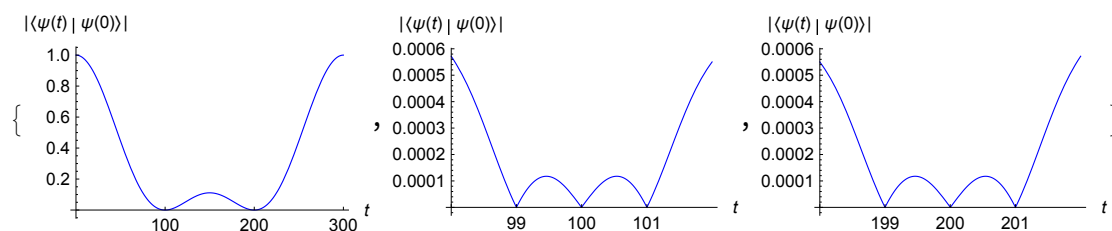

*Zeros of overlap with three almost-equal separations.* The first plot shows the magnitude of  $\langle\psi(t)|\psi(0)\rangle$  for one entire period of length  $T=300$ , for a state that minimizes  $T\Delta\nu$ ; the other two show details near  $t=100$  and  $200$ . What look like smooth minima in the first plot are each actually a triplet of zeros when we look closer. What's going on is that all states that are 99, 100 or 101 apart are mutually orthogonal,

so comparing with  $t=0$ , the overlap has zeros at three separations near 100, and at minus those separations. We also get zeros at separations that are a periodic sum of consecutive pairs of separations---but those are the same places again. Since only ratios of times matter in our minimizations, it's more meaningful to let the full period be our unit of time. Then the same evolution looks like this:

```
{ε = 2 / 300; plotOverlap[0, 1, 1, showMag, Ticks → {Range[3] / 3, Automatic}],
 plotOverlap[1 / 3 - ε, 1 / 3 + ε, 1, showMag, Ticks → {Range[3] / 3, Automatic}],
 plotOverlap[2 / 3 - ε, 2 / 3 + ε, 1, showMag, Ticks → {Range[3] / 3, Automatic}]}
```

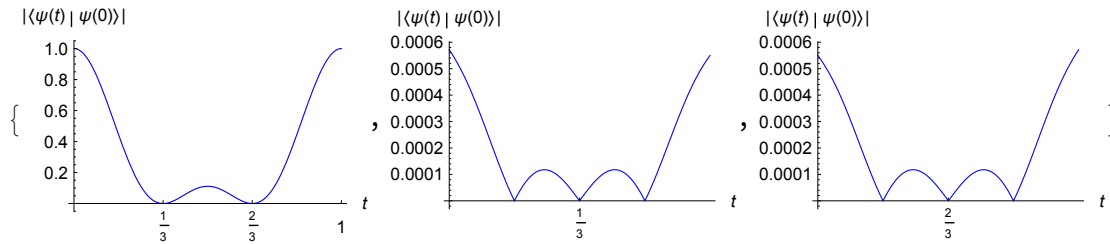

If we instead used {999, 1000, 1001} as our separations we would get something very similar, but with the detailed regions much reduced in width and height. In the limit, as we let the ratio of almost-equal separations approach one, we simply get an overlap with slope zero at  $1/3$  and  $2/3$ . In general, the almost-equal limiting points are obtained by performing a minimization with equal separations between  $K_{\text{different}}$  adjacent distinct states, adding the constraint at each zero of the overlap that the slope is also zero. **limitPlot** finds the almost-equal limiting minima in this manner, and plots them.

Extra “slope=0” constraints:

```
acosn := Table[{Sum[a_n n Cos[2 Pi n deltaList[[k]]], {n, 0, ntot - 1}} == 0},
 {k, 1, Length[deltaList]};
asinn := Table[{Sum[a_n n Sin[2 Pi n deltaList[[k]]], {n, 0, ntot - 1}} == 0},
 {k, 1, Length[deltaList]};
```

Construct table of differences between almost-equal limiting minima and exactly equal minima

```
limitTab[about_, moment_, kmin_, kmax_] := Block[{problem},
 ParallelTable[
 (problem := Flatten[{momTM, asum, apos, acos, asin, acosn, asinn}];
 2 minimizeTM[about, moment, Table[1, {n}], 2 n]) -
 (problem := Flatten[{momTM, asum, apos, acos, asin}];
 2 minimizeTM[about, moment, Table[1, {n}]]),
 {n, kmin, kmax}, Method → "FinestGrained"]]
```

```
limitPlot[about_, moment_, kmin_, kmax_] :=
 ListPlot[limitTab[about, moment, kmin, kmax],
 Joined → True, PlotStyle → blueDashed, DataRange → {kmin, kmax}]
```

```
blueDashed = Directive[Thickness[.0015], Blue, Dashing[ {.01, .005} ]];
```

For example, the straight line increase of minimum with number of different separations is exactly predicted by the limit of almost-equal separations (blue dashed line):

```
Show[minXPlot, limitPlot[aboutMin, 1, 1, 4]]
```

$T(\Delta v_{l,\min} - \Delta v_{\text{equal}})$

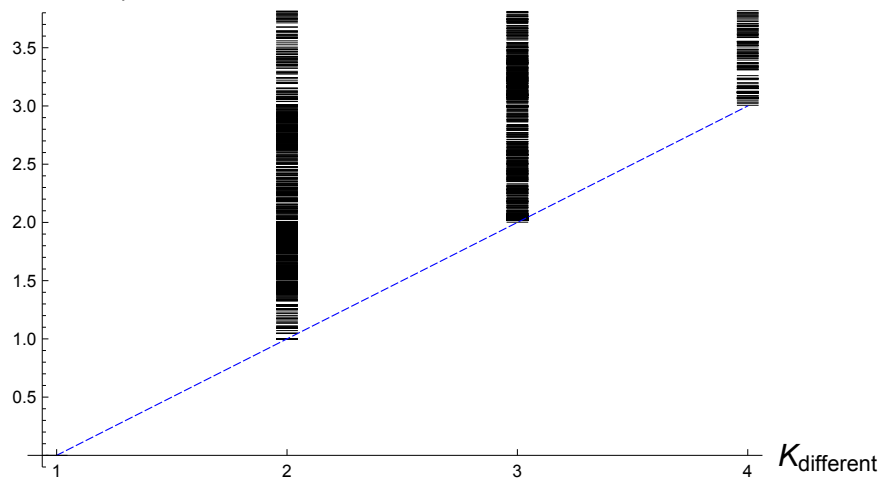

## Deviations from the mean

We run a similar but smaller experiment for the first moment about the mean.

```
mean2 = minimizeSets[aboutMean, 1, 2, 800];
```

Execution took 0.371 minutes

```
mean3 = minimizeSets[aboutMean, 1, 3, 800];
```

Execution took 1.246 minutes

```
mean4 = minimizeSets[aboutMean, 1, 4, 1100];
```

Execution took 4.056 minutes

```
meanXPlot = ListPlot[
```

```
  last2[Join[aeqList[aboutMean, 1, 4], aeqN[aboutMean, 1, 4], mean2, mean3, mean4]],
```

```
  PlotRange → {- .1, 0.698},
```

```
  PlotStyle → Black, Ticks → {Range[4], Automatic},
```

```
  PlotMarkers → Graphics[{Thickness[.03], Line[{{-.05, 0}, {.05, 0}}]}],
```

```
  AxesLabel → {Style["Kdifferent", 16], Style["T(Δvl,mean - Δvequal)", 16]};
```

Again, increase of minimum with number of different separations is predicted by the limit of almost-equal separations (blue dashed line):

```
Show[meanXPlot, limitPlot[aboutMean, 1, 1, 4], ImageSize -> 500]
```

$$T(\Delta V_{1,\text{mean}} - \Delta V_{\text{equal}})$$
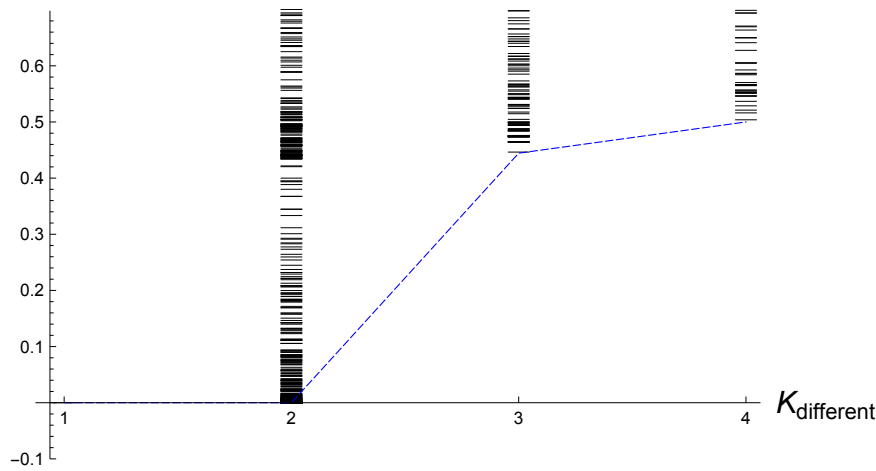

Equal separations ( $K_{\text{different}} = 1$ ) always gives the smallest global minimum, but for first moment deviations about the mean the  $K_{\text{different}} = 2$  case can come arbitrarily close. We investigate why that is:

```
mean2[[1]]
```

```
{{99, 100}, {1, 1}, 2, 0.0000623091}
```

```
minimizeTM[aboutMean, 1, {99, 100}]; makeOverlap;
```

```
{ε = .008; plotOverlap[0, 1, 1, showMag, Ticks -> {Range[2]/2, Automatic}],  
plotOverlap[1/2 - ε, 1/2 + ε, 1, showMag, Ticks -> {Range[2]/2, Automatic}]}
```

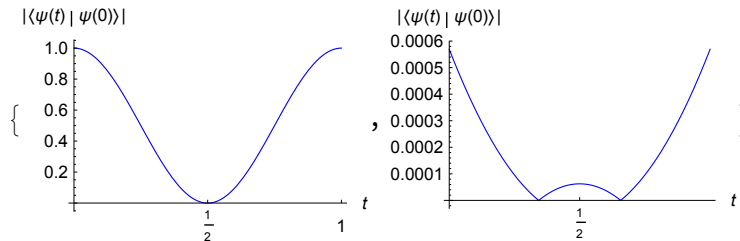

```
t =.; Total[overlap[t] / e^{198 i π t}]
```

```
0.499969 + 0.250016 e^{-2 i π t} + 0.250016 e^{2 i π t}
```

For this exceptional width, there are two different equally optimal states for two equal separations: one using two consecutive frequencies (equally weighted), and one using three. The latter is essentially the state shown above. Factoring out a phase (which doesn't affect the magnitude plotted), the left hand plot is a cosine scaled and shifted up, by adding a constant, to approximately touch the  $t$ -axis. The point where it touches has slope  $\approx 0$ , and so is the limiting solution. In the detailed plot (right hand) we see that the cosine is actually shifted down slightly to give two close-together zero crossings. Existence of this solution is related to the portion-bound for this width being lower than the periodic bound.

## Higher moments

Deviation-widths for other moments can be tested using these functions, and the almost-equal cases always give the smallest dimensionless widths  $T \Delta v$  for unequal separations. The limiting almost-equal plots for  $K_{\text{different}}$  from 1 to 10 with moments  $M$  between 1 and 10 are shown here for deviations about the minimum and about the mean. In all cases the lines get steeper as the moment increases:

```
Show[Table[limitPlot[aboutMin, m, 1, 10], {m, 1, 10}], Ticks → {Range[10], Automatic},
  AxesLabel → {Style["Kdifferent", 16], Style["T(ΔvM,min−Δvequal)", 16]}, ImageSize → 500]
```

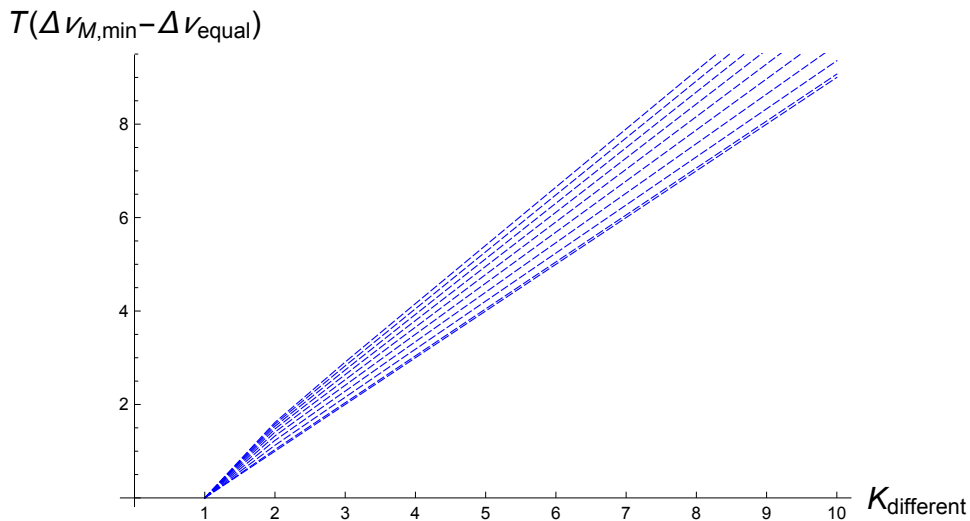

```
Show[Table[limitPlot[aboutMean, m, 1, 10], {m, 1, 10, 1/2}],
  Ticks → {Range[10], Automatic},
  AxesLabel → {Style["Kdifferent", 16], Style["T(ΔvM,mean−Δvequal)", 16]}, ImageSize → 500]
```

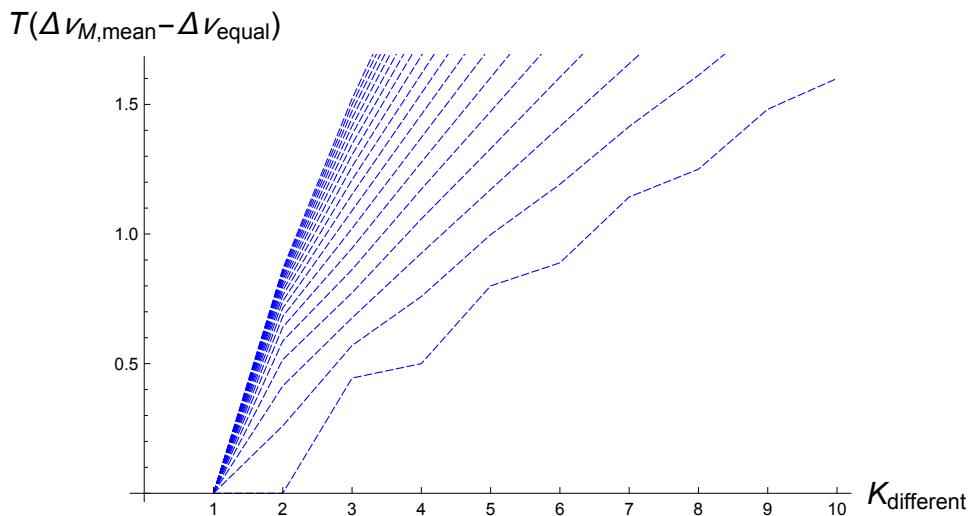

## Equal vs unequal separations in a portion of an evolution

We verify that, if we only know that there are  $\Delta N$  distinct states in a portion of length  $\Delta t$  of a much longer evolution (which may just be many repetitions of a periodic evolution), the minimum deviation widths are always smallest if the states are uniformly spaced within  $\Delta t$ . We do this by experimentally determining how minimum widths vary with the number  $K_{\text{different}}$  of different separation lengths in time  $\Delta t$ . We find, as in the periodic case, that the minimum possible widths increase in discrete jumps as  $K_{\text{different}}$  increases, so the global minimum is always obtained with equal separations.

Here we set the default maximum period of the evolution **pScale** to 100 times the length  $\Delta t$  of the portion. If we run with **pScale**=10 instead, the tests take an order of magnitude less time and, rescaled, the plots look almost the same.

```
pScale = 100;
```

To determine the minimum for a randomly chosen set of separations within a *portion* of length  $\Delta t$  we define **minimizeSetP**, which tests a specified set of separations. **randTauListP** is then used to generate a random list containing  $K_{\text{different}} = 2, 3$ , or 4 different separation lengths, each an integer up to 100.

```
randTauListP[ndiff_] := Module[{diff},
  diff = randDiffList[ndiff];
  RandomSample[Flatten[
    Table[diff[[n]], {n, 1, Length[diff]}, {If[RandomInteger[{1, 10}] < 10, 1, 2}]]]]
minimizeSetP[about_, moment_, tauList_, period_ : pScale] :=
  Block[{len, tl, el, osdMax = 3},
    {len = Length[tauList];
     tl = Join[tauList, Total[tauList] {period - 1}],
     el = Join[Table[1, {len}], len {period - 1}],
     Length[DeleteDuplicates[tauList]],
     -2 minimizeTM[about, moment, el] + 2 minimizeTM[about, moment, tl]]}
```

**minimizeSetsP** repeats **minimizeSetP** *numSets* times to construct a list of four element lists, and then prints out execution time.

```
minimizeSetsP[about_, moment_, ndiff_, numSets_, period_ : pScale] :=
  Module[{start, table},
    start = AbsoluteTime[];
    table = sortLast[ParallelTable[minimizeSetP[about, moment,
      randTauListP[ndiff], period], numSets, Method -> "FinestGrained"]];
    Print["Execution took ", Round[(AbsoluteTime[] - start) / 60, .01], " minutes"];
    table]
```

A usage example with **minimizeSetsP**. Results appear sorted by the value at the end of each element:

```
smallTestP = minimizeSetsP[aboutMin, 1, 3, 6]
```

```
Execution took 0.36 minutes
```

```
{{{98, 96, 95, 28611}, {1, 1, 1, 297}, 3, 185.14},
 {{100, 49, 90, 23661}, {1, 1, 1, 297}, 3, 273.87},
 {{100, 98, 42, 23760}, {1, 1, 1, 297}, 3, 297.753},
 {{100, 98, 35, 23067}, {1, 1, 1, 297}, 3, 304.284},
 {{99, 62, 99, 62, 100, 41778}, {1, 1, 1, 1, 1, 495}, 3, 416.883},
 {{14, 37, 19, 19, 8811}, {1, 1, 1, 1, 396}, 3, 418.819}}
```

```
last2[smallTestP]
```

```
{{3, 185.14}, {3, 273.87}, {3, 297.753}, {3, 304.284}, {3, 416.883}, {3, 418.819}}
```

## Deviations from the minimum

Now we run a randomized experiment to determine minimum possible values for the first deviation from a minimum frequency, for a portion of an evolution with  $K_{\text{different}}$  separations. We choose the number of samples tested for each  $K_{\text{different}}$  to get a reasonably even density of plotted points.

```
pmin2 = minimizeSetsP[aboutMin, 1, 2, 600];
```

```
Execution took 2.48 minutes
```

```
pmin3 = minimizeSetsP[aboutMin, 1, 3, 300];
```

```
Execution took 4.59 minutes
```

```
pmin4 = minimizeSetsP[aboutMin, 1, 4, 900];
```

```
Execution took 29.43 minutes
```

If we look at the minimum value of  $T\Delta v$  for each number  $K_{\text{different}} > 1$  of different separation lengths seen in a long experiment we find, as in the earlier periodic evolution case, that close-to-equal separations give the smallest minima for unequal separations. We also find this for other deviation widths.

```
{pmin2[[1, 1]], pmin3[[1, 1]], pmin4[[1, 1]]}
{{99, 100, 19701}, {98, 96, 97, 28809}, {97, 98, 96, 99, 38610}}
```

As in the full periodic evolution case, we compute a few extra minima here corresponding to almost-equal separations within  $\Delta t$  with higher resolution (larger integer numbers for the separations). **aeqP** tests *numSets* almost-equal sets of separations for each value of  $K_{\text{different}}$ , starting range at *start*

```
aeqP[about_, moment_, kMin_, kMax_, start_, extra_ : 1, numSets_ : 10] :=
  (Join@@sortLast[ParallelTable[
    minimizeSetP[about, moment, RandomSample[start + Range[k + extra], k]],
    {numSets}, {k, kMin, kMax}, Method -> "FinestGrained"]])
```

```
aeqP100Min = aeqP[aboutMin, 1, 3, 4, 100, 10, 20];
```

```
aeqP500Min = aeqP[aboutMin, 1, 3, 4, 500];
```

```

tString := ToString["T"_{pScale, TraditionalForm}];
pminXPlot =
ListPlot[last2[Join[{{1, 0}}, pmin2, pmin3, pmin4, aeqP100Min, aeqP500Min]],
  Ticks → {Range[4], Automatic}, PlotStyle → Black,
  PlotRange → {-.05, 1.3 Last[pmin4[[1]]]},
  PlotMarkers → Graphics[{Thickness[.03], Line[{{-.05, 0}, {.05, 0}]}]},
  AxesLabel → {Style["K_{different}", 16], Style[tString <> "(\Delta \nu_{I,min} - \Delta \nu_{equal})", 16]},
  ImageSize → 500]

```

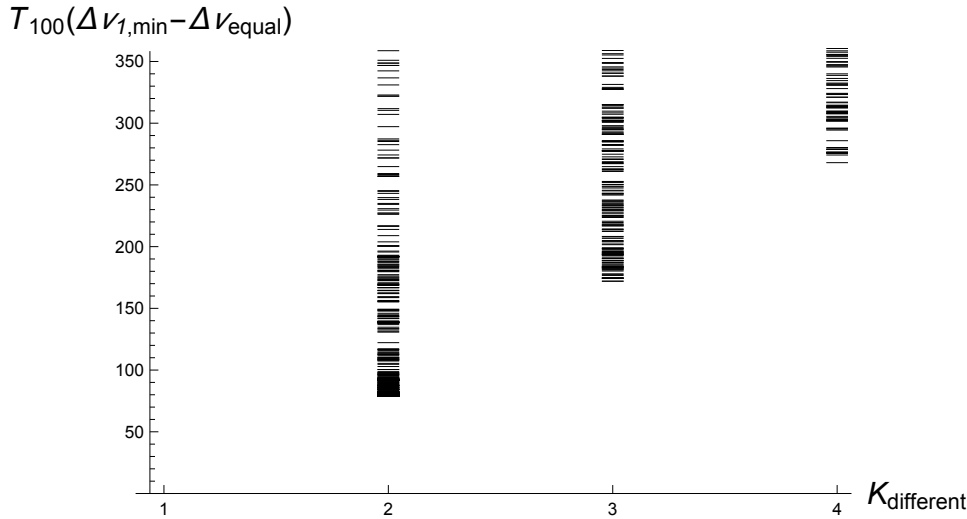

The smallest minima of  $T_{100}(\Delta \nu_{I,min} - \Delta \nu_{equal})$  for portions of evolution with different numbers of different separations  $K_{different}$  are nearly colinear. Equal separations ( $K_{different}=1$ ) give global minimum.

## Limiting behavior

Again we see that almost-equal separations define the smallest minima when separations are not exactly equal. If  $\tau$  is the average separation between adjacent distinct states in  $\Delta t$ , then with  $K$  different almost-equal separations between adjacent distinct states we get, in general,  $K$  zeros for the overlap  $\langle \psi(t) | \psi(0) \rangle$  for  $t$  near  $\tau$ , we get  $K-1$  near  $t=2\tau$ , etc. These are all the different separation lengths between any two distinct states. We can see this in the plots below, where for each list of separations the all-but-last set defines the contents of  $\Delta t$ , and the last separation is  $99 \Delta t$ , making the total period  $T=100 \Delta t$ . We make  $\Delta t$  our unit of time by setting the full period parameter  $t_{Full}$  of plotOverlap to 100, and plot the portion  $\Delta t$  and details near integer multiples of  $\tau$ .

```

minimizeTM[aboutMin, 1, {99, 100, 99 (99 + 100)}]; makeOverlap;

```

```
{ε = .01; plotOverlap[0, 1.05, 100, showMag, Ticks → {Range[2] / 2, Automatic}],
plotOverlap[1/2 - ε, 1/2 + ε, 100, showMag, Ticks → {Range[2] / 2, Automatic}],
plotOverlap[2/2 - ε, 2/2 + ε, 100, showMag, Ticks → {Range[2] / 2, Automatic}]}
```

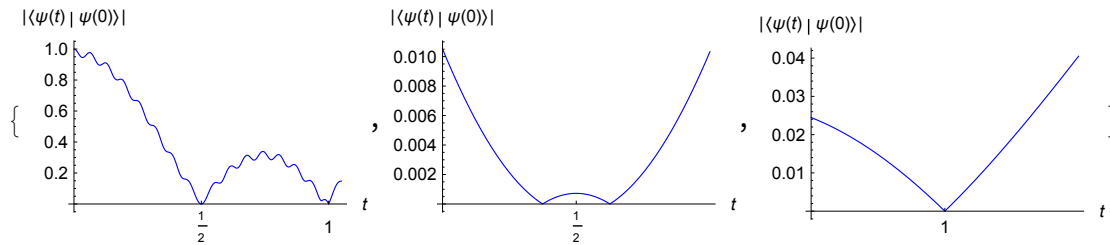

```
deltaList LCM@@Denominator[deltaList]
```

```
{99, 100, 199}
```

```
minimizeTM[aboutMin, 1, {98, 99, 97, 100, 99 (97 + 98 + 99 + 100)}]; makeOverlap;
```

```
{ε = .01; plotOverlap[0, 1.05, 100, showMag, Ticks → {Range[4] / 4, Automatic}],
plotOverlap[1/4 - ε, 1/4 + ε, 100, showMag, Ticks → {Range[4] / 4, Automatic}],
plotOverlap[2/4 - ε, 2/4 + ε, 100, showMag, Ticks → {Range[4] / 4, Automatic}],
plotOverlap[3/4 - ε, 3/4 + ε, 100, showMag, Ticks → {Range[4] / 4, Automatic}],
plotOverlap[4/4 - ε, 4/4 + ε, 100, showMag, Ticks → {Range[4] / 4, Automatic}]}
```

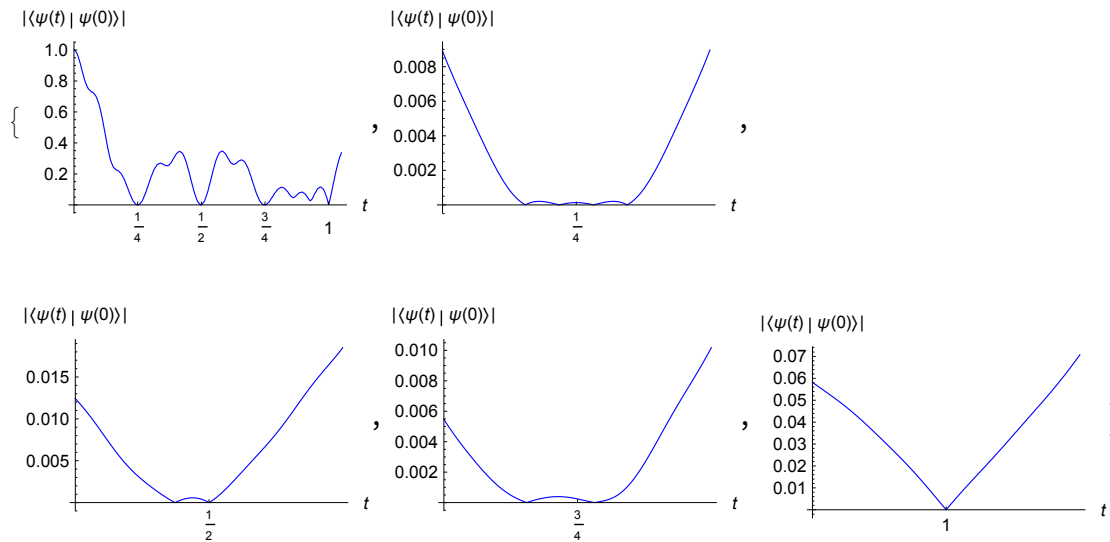

```
deltaList LCM@@Denominator[deltaList]
```

```
{97, 98, 99, 100, 196, 197, 294, 296, 394}
```

For the evolution with four almost-equal separations between adjacent distinct states, the full **deltaList** of separations where the overlap  $\langle \psi(t) | \psi(0) \rangle$  must be zero has four entries near 100, two near 200, two near 300, and only one near 400. The reason there are only two near 200 instead of three is because the adjacent-separation list {98, 99, 97, 100} has two adjacent pairs that add up to 197, giving one less orthogonal-separation constraint, allowing a reduced minimum. Nevertheless, all but the last multiple of 100 has more than one zero near it (there's only one way to get the last separation).

If we let the ratio of separations approach one, we converge to a situation in which we have equal separations between adjacent distinct states, but the overlap has  $\text{slope}=0$  at all but the last separation in **deltaList**. This is how we define the limit of almost-equal separations in general.

Extra  $\text{slope}=0$  constraints at all-but-largest distinct separations, for almost-equal limit:

```
acosnP := Table[{Sum[an n Cos[2 Pi n deltaList[[k]]], {n, 0, ntot - 1}} == 0},
  {k, 1, Length[deltaList] - 1}];
asinnP := Table[{Sum[an n Sin[2 Pi n deltaList[[k]]], {n, 0, ntot - 1}} == 0},
  {k, 1, Length[deltaList] - 1}];
```

**limitP** computes the difference between equal adjacent separations with the added  $\text{slope}=0$  constraint, and without it. It uses extra precision to get an accurate value. It also uses extra coefficients in the minimization, to accommodate the extra constraints.

```
limitP[about_, moment_, kdiff_, period_ : pScale] :=
  Block[{extraPrecision = 150, problem},
    Chop[(problem := Flatten[{momTM, asum, apos, acos, asin, acosnP, asinnP}];
      2 minimizeTM[about, moment,
        Join[Table[1, {kdiff}], kdiff {period - 1}], 10 kdiff period])
    - (problem := Flatten[{momTM, asum, apos, acos, asin}];
      2 minimizeTM[about, moment, Join[Table[1, {kdiff}], kdiff {period - 1}]])]
  limitTabP[about_, momentMin_, momentMax_, ndiffMin_, ndiffMax_, period_ : pScale] :=
    ParallelTable[limitP[about, moment, ndiff, period], {moment, momentMin, momentMax},
      {ndiff, ndiffMin, ndiffMax}, Method -> "FinestGrained"]
```

```
Show[pminXPlot,
  ListPlot[limitTabP[aboutMin, 1, 1, 1, 4], Joined -> True, PlotStyle -> blueDashed]]
```

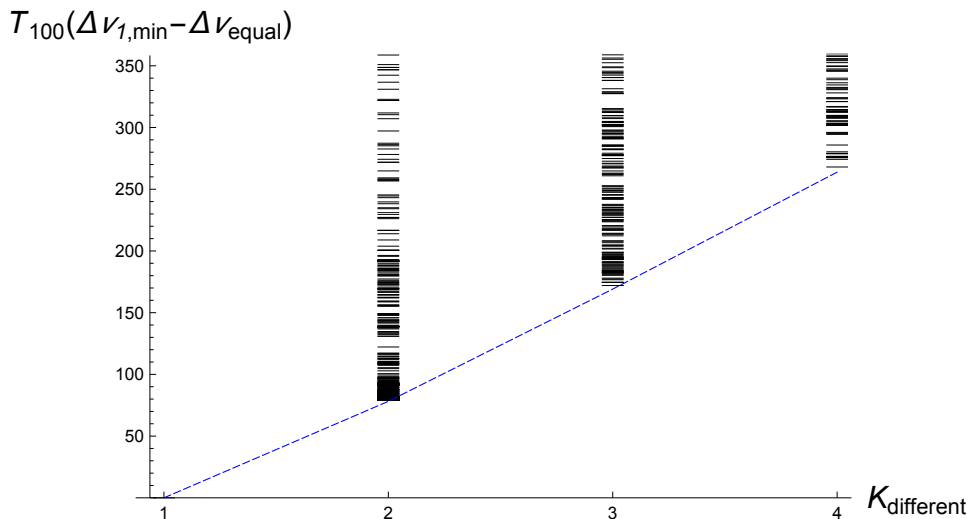

The smallest minima of  $T(\Delta\nu_{l,\min} - \Delta\nu_{\text{equal}})$  for  $K_{\text{different}}$  different separations between distinct states in a time interval  $\Delta t$  that is part of an evolution with period  $T = \text{pScale } \Delta t$  are bounded by the limit of almost-equal separations (blue dashed line). The global minimum corresponds to  $K_{\text{different}} = 1$ .

## Deviations from the mean

We run a similar experiment for the first moment about the mean.

```
pmean2 = minimizeSetsP[aboutMean, 1, 2, 400];
```

Execution took 12.18 minutes

```
pmean3 = minimizeSetsP[aboutMean, 1, 3, 300];
```

Execution took 30.07 minutes

```
pmean4 = minimizeSetsP[aboutMean, 1, 4, 700];
```

Execution took 161.61 minutes

```
aeqP100Mean = aeqP[aboutMean, 1, 3, 4, 100, 10, 20];
```

```
aeqP500Mean = aeqP[aboutMean, 1, 3, 4, 500];
```

```
pmeanXPlot =
```

```
ListPlot[Last2[Join[{{1, 0}}, aeqP500Mean, aeqP100Mean, pmean2, pmean3, pmean4]],
  Ticks → {Range[4], Automatic}, PlotStyle → Black,
  PlotRange → {- .05, 1.3 Last[pmean4[[1]]]},
  PlotMarkers → Graphics[{Thickness[.03], Line[{{- .05, 0}, {.05, 0}}]}],
  AxesLabel → {Style["Kdifferent", 16], Style[tString <> " $(\Delta \nu_{I, \text{mean}} - \Delta \nu_{\text{equal}})", 16]}$ , 16}},
  ImageSize → 500];
```

```
Show[pmeanXPlot,
```

```
ListPlot[limitTabP[aboutMean, 1, 1, 1, 4], Joined → True, PlotStyle → blueDashed]]
```

$T_{100}(\Delta \nu_{I, \text{mean}} - \Delta \nu_{\text{equal}})$

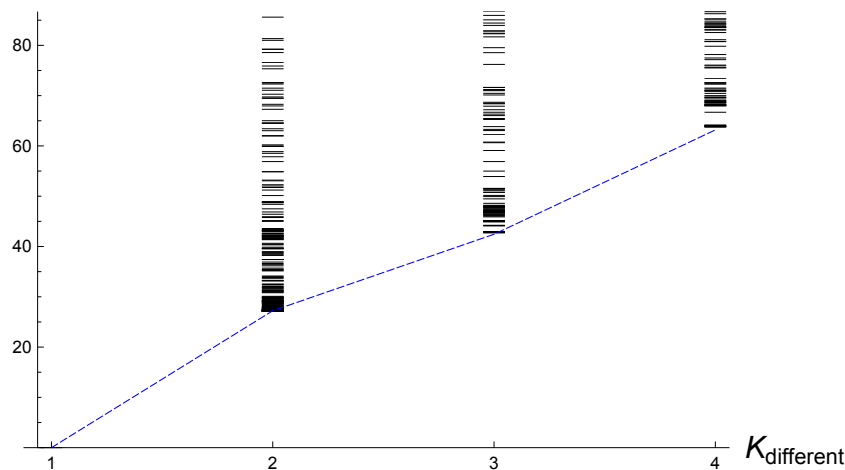

The smallest minima of  $T(\Delta \nu_{I, \text{mean}} - \Delta \nu_{\text{equal}})$  for  $K_{\text{different}}$  different separations between distinct states in a time interval  $\Delta t$  that is part of an evolution with period  $T = \text{pScale } \Delta t$  are bounded by the limit of almost-equal separations (blue dashed line). The global minimum corresponds to  $K_{\text{different}} = 1$ .

## Higher moments

Higher moments with unequal separations between adjacent distinct states are similarly bounded by almost-equal adjacent separations. We can summarize many long experiments by simply plotting the limit-bounds for higher moments. The limiting almost-equal plots for  $K_{\text{different}}$  from 1 to 8 with moments  $M$  from 1 to 10 are shown below for deviations about the minimum and about the mean. In all cases the lines get steeper as the moment increases:

```
limitMinTabs = limitTabP[aboutMin, 1, 10, 1, 8];
```

```
ListPlot[limitMinTabs, Joined → True, PlotStyle → blueDashed, ImageSize → 500,  
  AxesLabel → {Style[" $K_{\text{different}}$ ", 14], Style[tString <> " $(\Delta v_{M,\text{min}} - \Delta v_{\text{equal}})$ ", 14]}]
```

$T_{100}(\Delta v_{M,\text{min}} - \Delta v_{\text{equal}})$

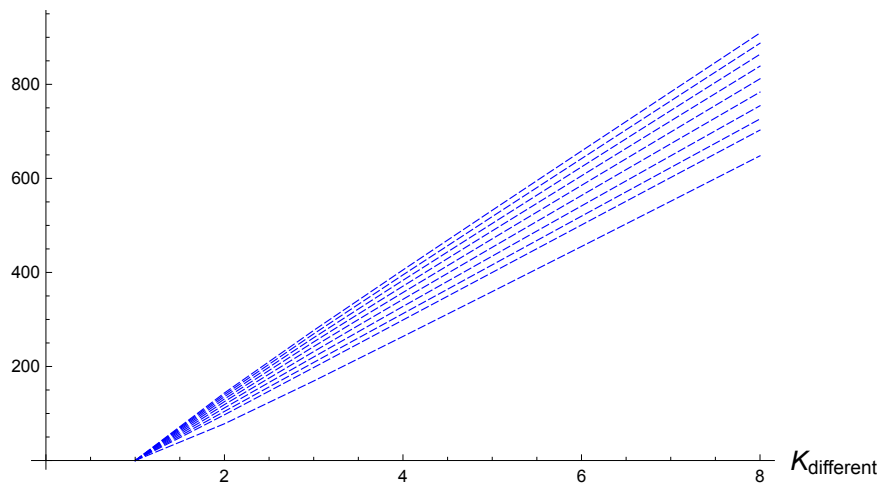

```
limitMeanTabs = limitTabP[aboutMean, 1, 10, 1, 8];
```

```
ListPlot[limitMeanTabs, Joined → True, PlotStyle → blueDashed, ImageSize → 500,  
  AxesLabel → {Style[" $K_{\text{different}}$ ", 14], Style[tString <> " $(\Delta v_{M,\text{mean}} - \Delta v_{\text{equal}})$ ", 14]}]
```

$T_{100}(\Delta v_{M,\text{mean}} - \Delta v_{\text{equal}})$

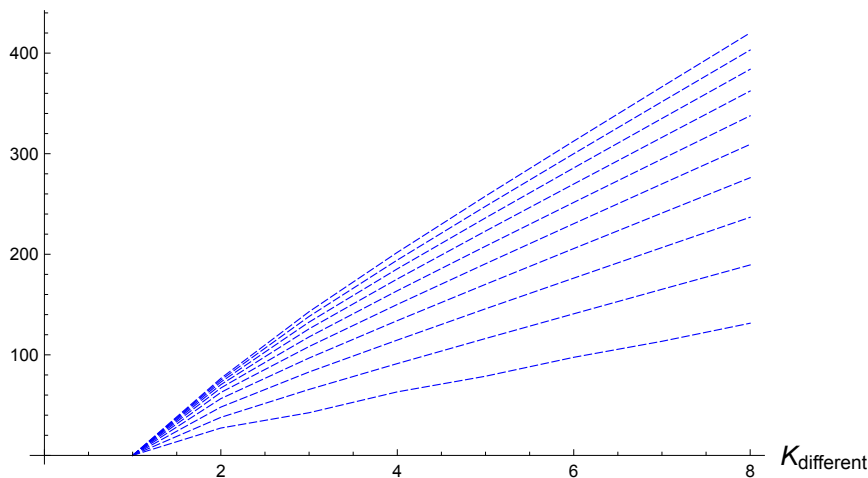

These graphs for almost-equal-separation limits are slightly different than the earlier ones for a complete periodic evolution. This is because having a particular value of  $K_{\text{different}}$  here is not the same constraint as it is for a periodic evolution. For example, we can have a total of just two separations in a periodic evolution, of different lengths, but if there are two different separations within a time  $\Delta t$  there must be at least three separations in the entire periodic evolution it is part of.

## Compare numerical and theoretical bounds

Assuming that equal separations between adjacent distinct states within a portion of an evolution allows the smallest possible dimensionless widths  $\Delta v \tau$ , we now compare theoretical bounds against numerical minima. We first define functions to produce plots of theory (solid) and numerical minima (dots) when the period is orders of magnitude longer than the portion. We use a prime number period so it isn't an integer multiple of any expected subperiod, letting us verify we really are seeing the length of the full period become irrelevant. Later we check for exact matches to 100 decimal digits when the period is 100 times as long as the expected minimum subperiod: any discrepancy would show up since the period is long enough to be almost irrelevant.

Since **minimizeTM** minimizes the period times the deviation,  $T\Delta v/2$ , multiplying by  $2\tau/T = 2/\text{period}$  gives the minimum for  $\tau\Delta v$ .

```
fNumerical[about_, m_, n_, period_] :=
  (2/period) minimizeTM[about, m, Join[Table[1, {n - 1}], {period - (n - 1)}]]

fTheory[about_, moment_, distinct_] :=
  If[about == aboutMin, fMin[moment, distinct], fMean[moment, distinct]];

plotTheory[about_, minM_, maxM_] :=
  Show[Plot[Table[fTheory[about, m, n], {n, {2, 3, 4, 6, 10, 30}}],
    {m, minM, maxM}, PlotStyle -> Directive[Blue, Thickness[.0015]],
    PlotRange -> {{0, 22}, All}, AxesLabel -> {Style["M", 16],
      If[about == aboutMin, Style["2<v-v_0>_M \tau", 16], Style["2<v-v_bar>_M \tau", 16]}]]];

fDataSets[about_, minM_, maxM_, incM_ : 1] := Transpose[ParallelTable[
  Block[{extraPrecision = 10 IntegerPart[m + 1 / m] + 3 n, osdMax = 0},
    fNumerical[about, m, n, 2003]], {m, minM, maxM, incM},
  {n, {2, 3, 4, 6, 10, 30}}, Method -> "FinestGrained"]];
```

## Deviations from the minimum

```
fDataMin = fDataSets[aboutMin, 1/2, 20, 1/4];
```

```
fMinInf[m_] = 2  $\left(\frac{1}{1+m}\right)^{1/m}$ ;
```

```
Show[plotTheory[aboutMin, 1/2, 20],  
Plot[fMinInf[m], {m, 1/2, 20}, PlotStyle → Directive[Blue, Thickness[.0015]]],  
ListPlot[fDataMin, PlotStyle → Directive[{PointSize[.006], Blue}],  
DataRange → {.5, 20}], AxesOrigin → {0, 0}, ImageSize → 600]
```

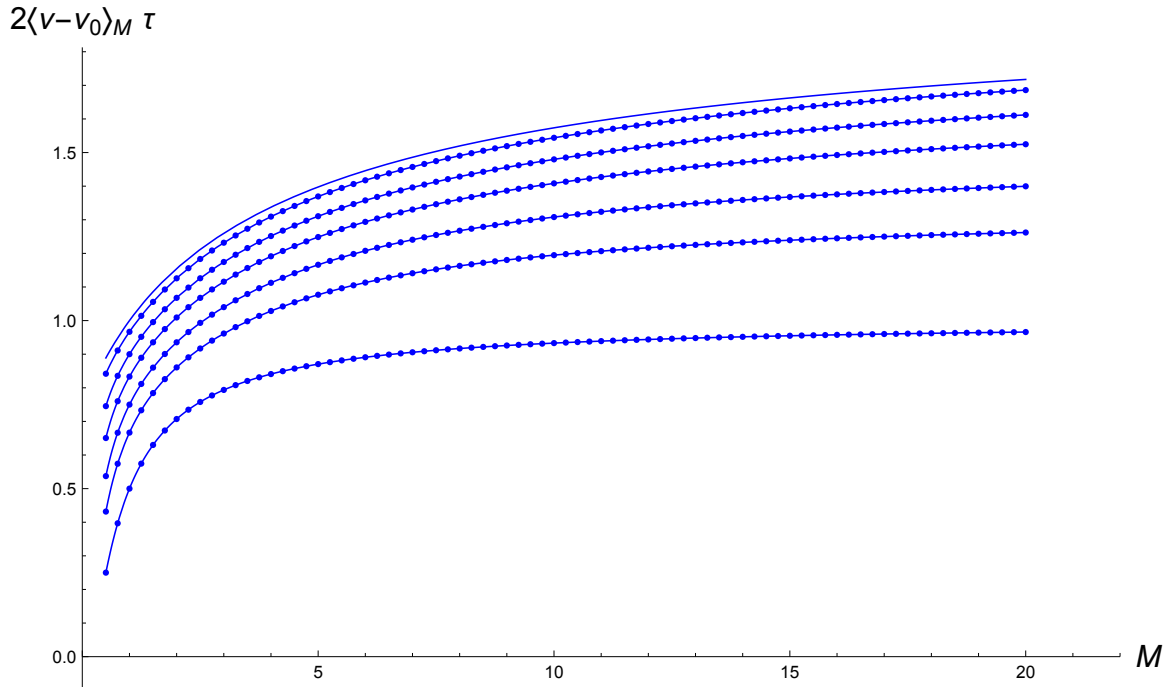

*Bounds on generalized deviations from a minimum frequency.* For long evolutions including a portion with  $\Delta N$  distinct states separated by  $\tau$ , minimum bandwidth bounds  $f_{v_0}(M, \Delta N)$  (solid) agree with numerical minima (dots). From bottom to top,  $\Delta N = 2, 3, 4, 6, 10, 30$  and  $\infty$ , with the last showing theory only. In this test we only verify convergence to the bounds when the period of the complete evolution is very large; we test exact limiting behavior below.

## Deviations from the mean

```
AbsoluteTiming[fDataMean = fDataSets[aboutMean, 2, 20, 1 / 4];]
{449.181, Null}
```

$$fMeanInf[m_] = \left( \frac{1}{1+m} \right)^{1/m};$$

```
Show[plotTheory[aboutMean, 2, 20],
Plot[fMeanInf[m], {m, 2, 20}, PlotStyle → Directive[Blue, Thickness[.0015]]],
ListPlot[fDataMean, PlotStyle → Directive[{PointSize[.006], Blue}],
DataRange → {2, 20}], AxesOrigin → {0, .45}, ImageSize → 600]
```

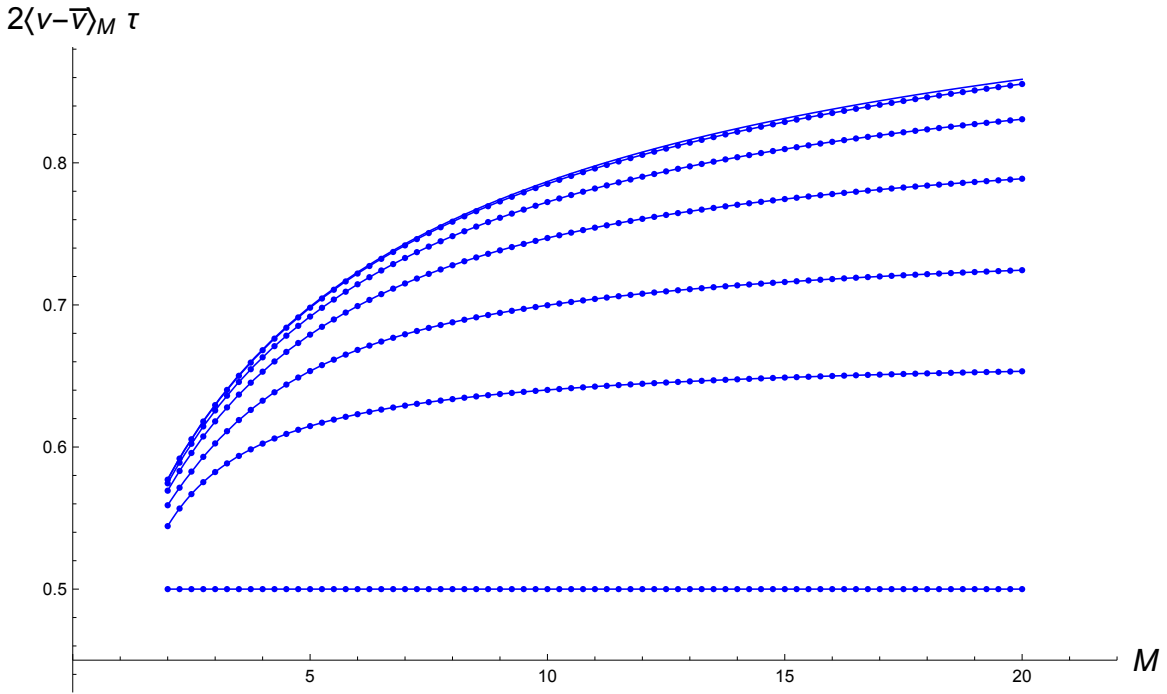

*Bounds on generalized deviations from a mean frequency.* For long evolutions including a portion with  $\Delta N$  distinct states separated by  $\tau$ , minimum bandwidth bounds  $f_{\bar{v}}(M, \Delta N)$  (solid) agree with numerical minima (dots). From bottom to top,  $\Delta N = 2, 3, 4, 6, 10, 30$  and  $\infty$ , with the last showing theory only. Again, here we only verify convergence to the bounds when the period of the complete evolution is very large; we test exact limiting behavior below.

## Confirm the match is exact

We compare each value from a minimization for the period  $100 N\tau$  with the values predicted by  $f_\alpha(M, N)$ . We verify that all comparisons are equal to more than 100 decimal digits. Comparing many digits can be considered a statistical test to verify the values are exactly equal, without algebraically proving it. Rerun these tests with **extraPrecision** = 1200 in **checkAMN** to verify exact agreement to 1000 digits (takes three times as long).

```
checkAMN[about_, m_, n_, k_] :=
  Block[{extraPrecision = 200},
    Abs[fTheory[about, m, n] - fNumerical[about, m, n, k n]]]
```

First verify that the periodic-bound **fTheory** has a non-zero difference from the numerical portion-bound in a case where we expect that: first-moment deviations from the mean for  $\Delta N=2$  distinct states.

```
checkAMN[aboutMean, 1, 2, 100]
0.0607127889771660955674785391380935449438958563866701416819326823240477872897528\
83269651802078420318712634110556656281816121121499495922774200494071114682757092\
74815451654356649075786091557540016935
```

Now test about a thousand cases about the mean, and a thousand about the minimum, where we expect the bounds to be the same. All differences between periodic and portion bounds are zero to more than 100 digits.

```
AbsoluteTiming[
  checkMin = ParallelTable[checkAMN[aboutMin, m, n, 100], {m, 1, 30}, {n, 2, 30}];]
{2117.07, Null}
```

```
{Max[checkMin], Accuracy[checkMin]}
{0. × 10-128, 127.827}
```

```
AbsoluteTiming[
  checkMean = ParallelTable[checkAMN[aboutMean, m, n, 100], {m, 2, 30}, {n, 2, 30}];]
{6730.29, Null}
```

```
{Max[checkMean], Accuracy[checkMean]}
{0. × 10-120, 119.536}
```

## Minimum widths for a portion as full period varies

We define a function **wTabAMList** which takes a given list of intervals, and applies **minimizeTM** to a sequence of lists derived from this, each with a single additional interval of increasing size appended to the given list. **wTabAMList** prepares a table of all information needed to plot minima for a range of values of the total period  $T$ . We plot  $2\tau \langle v - \alpha \rangle_M = (2\tau / T) T \langle v - \alpha \rangle_M$ , with  $\tau$  the average interval size, showing absolute or relative minima. **wTabAMN** runs **wTabAMList** on  $N$  equal intervals.

```
wTabAMList[about_, moment_, tauList_, start_ : 0, repeat_ : repeat] :=
  Block[{tt, intervals, tauAvg, minExtra, wTab, osdMax = 9},
    tt = Total[tauList];
    intervals = Length[tauList];
    tauAvg = Ceiling[tt / intervals];
    minExtra = Max[tauAvg (start - intervals), Ceiling[tauAvg / 4]];
    wTab =
      ParallelTable[ ((2 tauAvg / (tt + n)) minimizeTM[about, moment, Join[tauList, {n}]]),
        {n, minExtra, ((intervals + 1) repeat - intervals) tauAvg}];
    {Join[Table[Max[wTab], {minExtra}], wTab], about, moment, intervals + 1}]

wTabAMN[about_, moment_, distinct_, start_ : 0, repeat_ : repeat, tauL_ : tauL] :=
  wTabAMList[about, moment, Table[tauL, {distinct - 1}], start, repeat]

tauL          default number of points plotted per separation interval
repeat         default maximum total period to test = repeat * N * tau
widthLabels    an AxesLabel specification for ListPlot, with  $2 \langle v - \alpha \rangle \tau$  and  $T/\tau$  as the labels
noLabels       an AxesLabel specification for ListPlot
plotAbs        plot the absolute minimum value of  $2 \langle v - \alpha \rangle \tau$  for each value of  $T/\tau$ 

tauL = 43; repeat = 5; (* Default values *)

plotAbs[tabArgs_, labelFn_ : noLabels, maxRange_ : .08, yOffset_ : -1] :=
  Module[{wTab, about, moment, distinct, wMax, wMin, offset},
    {wTab, about, moment, distinct} = tabArgs; wMax = Max[wTab]; wMin = Min[wTab];
    offset = If[yOffset < 0, .05 maxRange, yOffset];
    ListPlot[wTab, Filling -> wMin, DataRange -> {distinct - 1, distinct repeat},
      Joined -> True, PlotRange -> {wMin - offset, wMin + 1.05 maxRange},
      AxesOrigin -> {0, wMin - offset}, Ticks -> {distinct Range[0, repeat], Automatic},
      AxesLabel -> labelFn[moment, about], PlotTheme -> "Classic"]

widthLabels[moment_, about_] := {Style["T/tau", 16],
  Row[{Style[Subscript[If[about == aboutMean, "2 <v - v-bar>", "2 <v - v_0>"],
    Style[moment, FontSize -> Small]], 16], Style["tau", 16]}]}

noLabels[moment_, about_] := None
```

## Examples of variation of minimum $\Delta v \tau$ as $T/\tau$ varies

The full evolutions that minimize  $\Delta v \tau$  are periodic, given that a portion with average separation  $\tau$  contains  $N$  distinct states. If we minimize  $\Delta v \tau$  for different values of the total period  $T$ , we can see this periodicity: global minima repeat. We can also see how the variation of the minima decreases as the total period increases. In fact, **wTabAMN** can be used to show that the variation always decreases like  $T^{-2}$  for large  $T$ , for any deviation width with a finite moment  $M$ . Here we only provide some examples illustrating that numerical global minima obtained by varying  $T$  agree with theory:

```
Table[plotAbs[wTabAMN[aboutMin, 1, n], widthLabels, .08, .01], {n, 2, 4}]
```

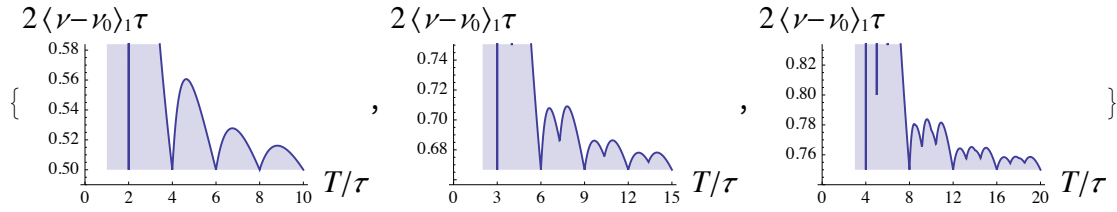

```
N[Table[{Min[wTabAMN[aboutMin, 1, n][[1]]], fMin[1, n]}, {n, 2, 4}]]
```

```
{{0.5, 0.5}, {0.666667, 0.666667}, {0.75, 0.75}}
```

```
Table[plotAbs[wTabAMN[aboutMean, 2, n], widthLabels, .04, .005], {n, 2, 4}]
```

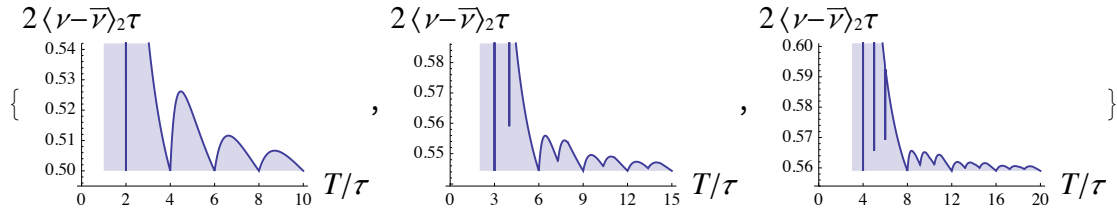

```
N[Table[{Min[wTabAMN[aboutMean, 2, n][[1]]], fMean[2, n]}, {n, 2, 4}]]
```

```
{{0.5, 0.5}, {0.544331, 0.544331}, {0.559017, 0.559017}}
```

## An exceptional case

The deviation-width bounds on entire periodic evolutions with a given number of distinct states generally agree with the bounds on portions, if both are expressed in terms of average separation between distinct states. This is not true, however, for some deviations about the mean for moments  $M < 2$  and an even number  $N$  of distinct states. Here we consider the case  $N=2$ :

```
wMean1n2 = wTabAMN[aboutMean, 1, 2];
Show[plotAbs[wMean1n2, widthLabels],
  Ticks -> {2.7 Range[0, 4], Automatic}, ImageSize -> 400]
```

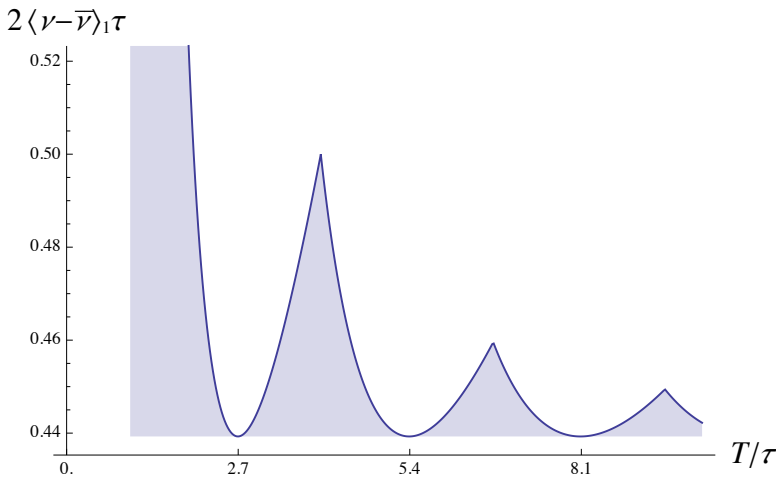

*Minimum of  $\Delta \nu \tau$  as  $T/\tau$  varies.* We numerically find the minimum of  $2 \langle \nu - \bar{\nu} \rangle_1 \tau$  for two distinct states with separation  $\tau$  in a total period  $T$ , for a range of values of  $T$ . The theoretically predicted global minimum recurs at the theoretically predicted  $T/\tau$ .

The measured minimum is:

```
Min[wMean1n2[[1]]]
0.439284
```

We get exactly the same result from our theoretical calculation of minimum deviation widths about the mean with  $\Delta N=2$  and  $M < \pi/2$ . The period is given by a transcendental equation. For  $M=1$ , we have

```
periodT = tt /. FindRoot[ $\frac{2 \pi / tt}{\tan[\pi / tt]} == 1$ , {tt, 2}]
2.69535
```

The minimizing distribution has probability **probT** for the two frequencies that are adjacent to the mean (i.e., that differ from it by  $1/\mathbf{periodT}$ ). This defines the minimum of  $\Delta \nu \tau$ :

```
probT =  $\frac{1}{4 \sin[\pi / \mathbf{periodT}]^2}$ ; deltaNuTauMin = 4 probT / periodT
0.439284
```

## Threshold for exceptions to **fMean** for a portion

Bounds on portions always increase with the number of distinct states  $\Delta N$  in the portion. Bounds on periodic evolutions may not: this happens for some  $M < 2$  deviations about the mean with  $N$  even. The two kinds of bounds must agree above some threshold value of  $M$ . The threshold where the difference  $\Delta f_N$  between the two kinds of bounds becomes zero is  $M = \pi/2$  for  $N=2$  and increases with  $N$ :

```
ParallelTable[Plot[fMean[m, n] - fNumerical[aboutMean, m, n, 100 n], {m, 1.45, 2},
  PlotRange -> {-10^-7, 4.9 x 10^-6}, AxesLabel -> {"M", "Δf"_n}, PlotStyle -> Blue],
  {n, 2, 6, 2}, Method -> "FinestGrained"]
```

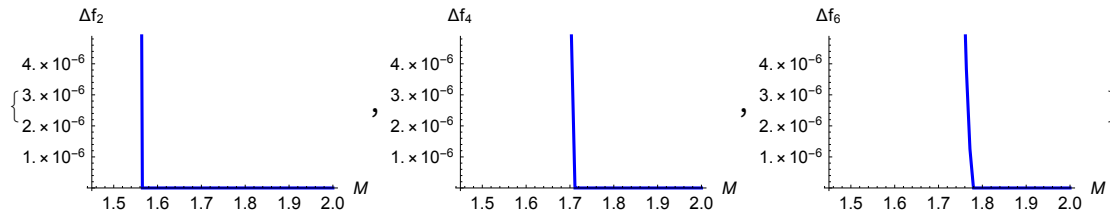

Odd- $N$  periodic bounds are always correct portion bounds. We determine the maximum threshold is  $M=2$  by seeing when periodic bounds **fMean** for even- $N$  converge to the average of the adjacent always-correct odd- $N$  **fMean** bounds. This happens for  $N \rightarrow \infty$ . We exhibit this numerically for  $N=100,000$ .

```
Block[{n = 100 000}, Plot[fMean[m, n] - fMean[m, n + 1] / 2 - fMean[m, n - 1] / 2,
  {m, 1.9, 2.7}, WorkingPrecision -> 100, PlotPoints -> 100, MaxRecursion -> 4,
  PlotStyle -> Blue, PlotRange -> {-1.2 x 10^-17, 8.8 x 10^-17}, AspectRatio -> .45,
  AxesLabel -> {Style["M", 16], Style["f_even - f_bar_odd", 16]}, ImageSize -> 500]]
```

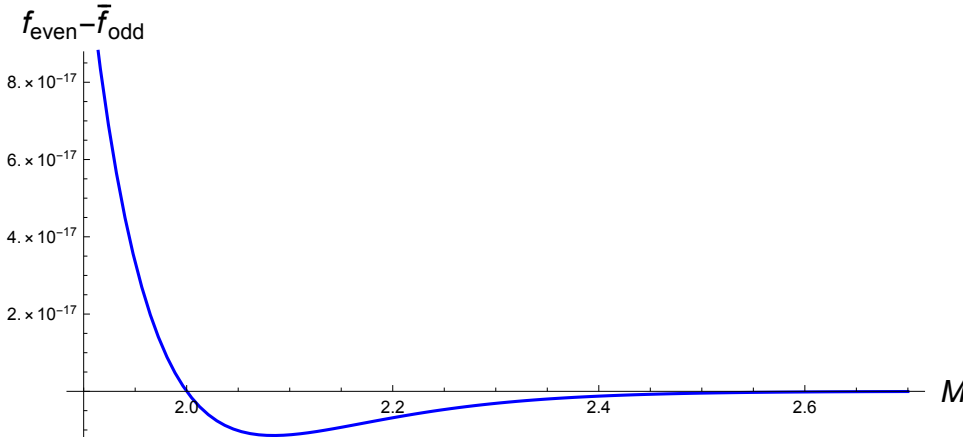

*Threshold for exceptions to minimum bandwidth.* The smallest  $M$  above which the minimum bandwidth bound  $f_{\nabla}(M, N)$  holds for a portion with even  $N$  increases with  $N$ , with a limiting value of 2. We see here that when  $M \lesssim 2$ ,  $f_{\text{even}} \equiv f(N) > \bar{f}_{\text{odd}} \equiv (f(N+1) + f(N-1))/2$ . The average  $\bar{f}_{\text{odd}}$  of correct odd- $N$  bounds approximates a correct even- $N$  bound, becoming exact as  $N \rightarrow \infty$ . Here  $N$  is  $10^5$ .

# Probability in a Frequency Range

## Frequency-range bounds for portion of a longer evolution

**maximizeFR** uses the same constraints as **minimizeTM**, but instead maximizes the sum of probabilities in a frequency *range* for the list of separations *sepList* between consecutive distinct states. *range* is the number of consecutive frequencies within which we will maximize probability. **ntot** is the integer period of the evolution given by the total of *sepList*, normalized so separations are integers. This is also the number of distinct frequencies and phases, hence number of coefficients  $a_n$  to be determined.

```
rProblem := Flatten[{rsum, asum, apos, acos, asin}];
rsum := {Sum[an, {n, 0, nrange - 1}]}];

maximizeFR[range_, sepList_] := Module[{d}, nrange = range;
  tauList = sepList / Total[sepList]; ntot = LCM @@ Denominator[tauList];
  deltaList = Sort[DeleteDuplicates[Flatten[Table[Min[d = (t[m] - t[k]), 1 - d],
    {k, 0, Length[tauList] - 2}, {m, k + 1, Length[tauList] - 1}]]]];
  soln = NMaximize[rProblem, vars]; soln[[1]]]
```

**qMaxL** determines the maximum total probability  $q$  that can be attached to a range of consecutive frequencies of width *delta*, given the evolution includes a portion with Length[*plist*]+1 *distinct* states with integer separations *plist*. We normalize *plist* to have average separation  $\tau = 1$ , then determine a maximum *period* (which defines the discrete frequency spectrum) to be some number of *cycles* of length *distinct* plus an *offset*. Since allowed frequencies are  $1/\text{period}$  apart, the width *delta*  $\geq (\text{range}-1)/\text{period}$ , where *range* is the largest integer number of frequencies that fit into *delta*.

```
qMaxL[plist_, delta_, cycles_ : 1, offset_ : 0] :=
  Module[{distinct, period, extra, range, tlist}, distinct = 1 + Length[plist];
  period = cycles distinct + offset; range = 1 + Floor[delta period];
  tlist = Join[plist Length[plist] / Total[plist], {1 + period - distinct}];
  maximizeFR[range, tlist]]
```

**qMax** is a special case of **qMaxL** where the distinct states are equally separated, and we specify only the number *distinct* of them, rather than a list of separations *plist*.

```
qMax[distinct_, delta_, cycles_ : 1, offset_ : 0] :=
  qMaxL[Table[1, distinct - 1], delta, cycles, offset];
```

**qMaxR** is a special case of **qMaxL** where a *plist* with a number *distinct* of elements is constructed randomly, using integer separations ranging from 1 to 10, with unit separations the most likely.

```
qMaxR[distinct_, delta_, cycles_ : 1] := (
  pl = Table[If[RandomInteger[{0, distinct}] < distinct, 1, RandomInteger[{1, 10}]],
    distinct - 1]; qMaxL[pl, delta, cycles])
```

## Width of frequency range vs. probability within range

We perform 10,000 maximizations of probability within randomly chosen frequency ranges for random sets of separations in a periodic evolution, and compare the result to the theoretical global maximum. The minimum width for given probability corresponds to the maximum probability for given width.

```
nmax = 10; tx = ParallelTable[nn = RandomInteger[{2, nmax}];
  del = RandomInteger[{0, 40}] / 20; {qMaxR[nn, del, 1] nn, del nn}, {10 000}];

pl = Plot[Ceiling[q] - 1, {q, 0, nmax}, PlotStyle -> Directive[Thickness[.001], Blue],
  ImageSize -> Full, AxesLabel -> {Style["q N", 16], Style["Δv τ N", 16]}];

ptx = ListPlot[tx, ImageSize -> Full, PlotStyle -> Directive[{PointSize[.006], Black}]];

Show[pl, ptx, PlotRange -> {{0, 4.91}, {0, 10}}, ImageSize -> 600]
```

$\Delta v \tau N$

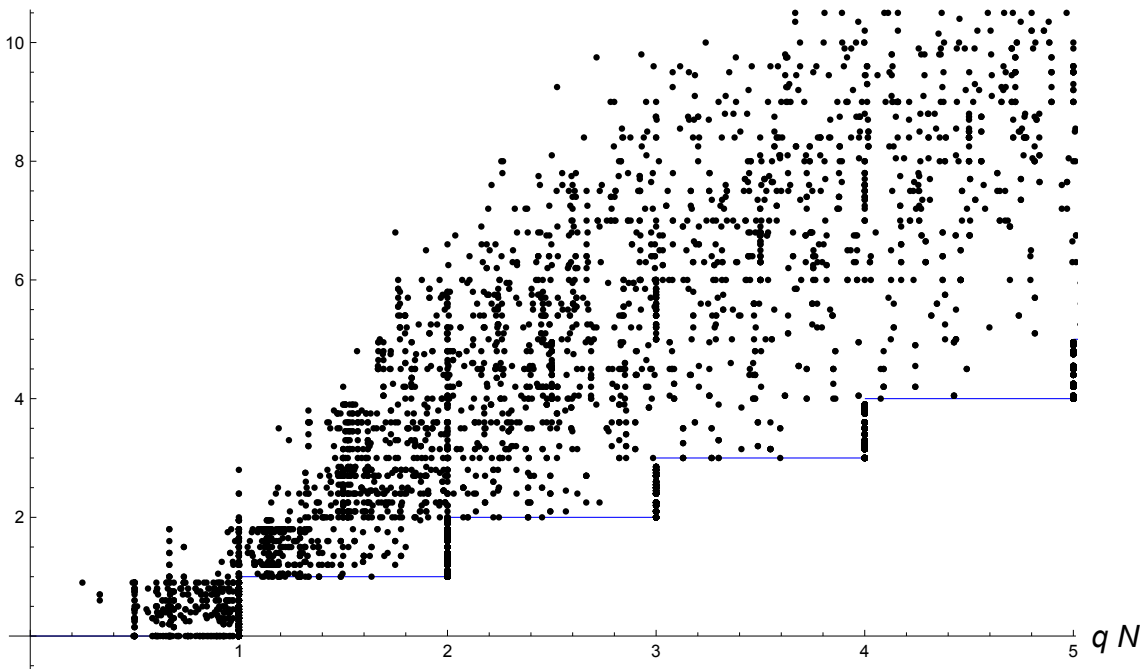

*Width of frequency range vs. probability within range.* Each dot shown represents a periodic evolution with  $N \leq 10$  distinct states, with separations and width  $\Delta v$  both chosen randomly. Maximum probability  $q$  in chosen  $\Delta v$  is found numerically. Blue is the theoretical bound.

## Compare numerical and theoretical bounds

Assuming equal separations are optimal, we compare numerical frequency widths  $\Delta v_q$  needed to hold probability  $q$ , for an evolution with a portion containing  $\Delta N$  distinct states, with theoretical bounds.

```
tMax2 = ParallelTable[{qMax[2, j/50, 200], j/50}, {j, 0, 25}];
tMax5 = ParallelTable[{qMax[5, j/75, 100], j/75}, {j, 0, 60}];
tMax30 = ParallelTable[{qMax[30, j/60, 100], j/60}, {j, 0, 58}];

pM[table_] := ListPlot[table, PlotStyle -> Directive[{PointSize[.006], Blue}]];

phu2 =
  Plot[1/π ArcCos[1/q - 1], {q, 1/2, 1}, PlotStyle -> Directive[Thickness[.0006], Blue]];

pLin[distinct_] := Plot[If[q < 1/distinct, 0, q - 1/distinct], {q, 0, 1},
  PlotStyle -> Directive[Thickness[.0006], Blue]];

Show[pLin[30], pM[tMax30], pLin[5], pM[tMax5], pLin[2], pM[tMax2], phu2,
  AxesLabel -> {Style["q", 16], Style["Δv_q τ", 16]}, ImageSize -> 600]
```

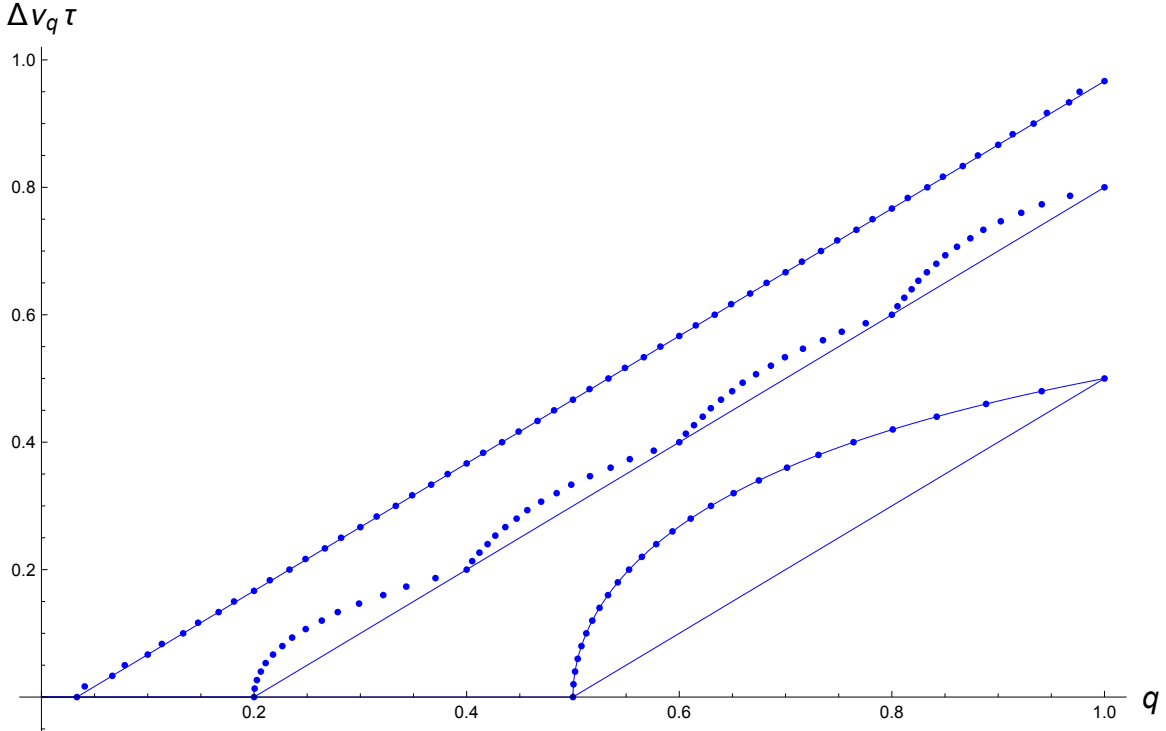

*Probability range bounds.* For a long evolution that includes  $\Delta N$  distinct states separated by  $\tau$ , a minimum range  $\Delta v_q$  is needed to hold probability  $q$ . We illustrate three cases:  $\Delta N=30$  (upper),  $\Delta N=5$  (middle) and  $\Delta N=2$  (lower). Dots are numeric minima, the curved line is a tight theoretical bound for  $\Delta N=2$ , and straight lines are the best linear bounds  $\Delta v_q \tau = q - 1/\Delta N$  that hold for a complete periodic evolution. We see the linear bounds are already a very good approximate bound at  $\Delta N=30$ .

## Equal separations in a portion allow minimum bandwidth

First we perform a short test to illustrate that, with equal separations  $\tau = 1$  between  $\Delta N$  distinct states in a portion that is 1% of the total period,  $(\Delta N - 1)/\Delta N$  is the minimum bandwidth. Even 99.9% of this bandwidth is insufficient to hold a total probability of one.

```
ParallelTable[{qMax[n, (n - 1) / n, 100], qMax[n, .999 (n - 1) / n, 100]}, {n, 2, 30}]
{{1., 0.984534}, {1., 0.991038}, {1., 0.993564}, {1., 0.99495},
 {1., 0.995834}, {1., 0.996451}, {1., 0.996907}, {1., 0.997258}, {1., 0.997537},
 {1., 0.997764}, {1., 0.995976}, {1., 0.996289}, {1., 0.996556}, {1., 0.996788},
 {1., 0.99699}, {1., 0.997168}, {1., 0.997326}, {1., 0.997467}, {1., 0.997594},
 {1., 0.997709}, {1., 0.99677}, {1., 0.996911}, {1., 0.99704}, {1., 0.997158},
 {1., 0.997268}, {1., 0.997369}, {1., 0.997464}, {1., 0.997551}, {1., 0.997633}}
```

Now we show that if separations between  $\Delta N$  distinct states in a portion are **not equal**, bandwidth  $\Delta v$  and average separation  $\tau$  obey  $\Delta v \tau > 1$ . Since we can achieve  $\Delta v \tau = (\Delta N - 1)/\Delta N < 1$  in a periodic evolution with equal separations, only equal separations allow minimum  $\Delta v \tau$ . With even one extra constraint, unequal separations do not allow all probability to fit into a frequency range of width  $1/\tau$ :

```
Table[qMaxL[{1, 1, 1, 1, 1, 2}, 1, cycles], {cycles, {100, 1000, 10 000}}]
{0.963224, 0.963229, 0.963229}
```

A period of length  $100 \Delta N \tau$  gives about 6 digits of precision. Now we try 30 sets of **unequal** random separations, reusing **randTauList** from the first statistical experiment at the beginning of the notebook to produce the sets. In no case can all probability fit into a frequency range of width  $1/\tau$ .

```
randTau := If[RandomInteger[1] == 0, RandomInteger[{1, 3}], RandomInteger[{1, 10}]];
rtl = Table[randTauList[RandomInteger[{2, 4}]], 30]
{{8, 3, 3, 9, 1, 3}, {4, 4, 3, 3, 7}, {8, 1}, {6, 3, 5}, {6, 6, 3, 7, 6, 3, 1},
 {9, 1, 3}, {9, 1}, {1, 1, 6}, {4, 4, 1, 4, 9, 3}, {2, 2, 4, 2, 9, 3},
 {2, 9, 7, 10}, {2, 3, 3}, {2, 3}, {3, 3, 1, 4, 2, 3}, {1, 3, 2}, {5, 7, 2, 1},
 {3, 1, 9, 1, 9, 3, 1}, {10, 4, 4, 1, 2}, {1, 6, 2, 1, 5, 1, 2}, {1, 10},
 {1, 3, 3, 5}, {1, 10, 3}, {2, 9, 2, 2}, {3, 2, 1, 2}, {9, 7, 9, 8, 7, 3, 8, 9},
 {3, 2}, {2, 6, 1, 8, 8, 6, 8, 2}, {3, 2, 6, 1}, {3, 8, 3}, {2, 4, 9}}
```

```
Max[ParallelTable[qMaxL[r, 1, 100], {r, rtl}]]
0.927044
```

Finally, we repeat this test for 10,000 cases.

```
rtl = Table[randTauList[RandomInteger[{2, 4}]], 10 000];
Max[ParallelTable[qMaxL[r, 1, 100], {r, rtl}]]
0.970257
```

A wide variety of similar tests verify bandwidth  $\Delta v > 1/\tau$  for a portion with unequal separations.

---

## End of tests

```
Print["Evaluation took ", Round[(AbsoluteTime[] - beginTime) / 3600, .1], " hours."]
```

```
Evaluation took 8.8 hours.
```
